# Supplementary material for: Predicting neutron experiments from first principles: A workflow powered by machine learning
Source: arXiv:2504.19352 ancillary file (2025-04-27)
Supplement: Supplementary file 1 [file supporting-information.pdf]

# Supporting Information

## Predicting neutron experiments from first principles: A workflow powered by machine learning

Eric Lindgren[1], Adam Jackson[2], Erik Fransson[1], Esmée Berger[1], Goran Škoro[1], Svemir Rudić[1], Rastislav Turanyi[2], Sanghamitra Mukhopadhyay[3], and Paul Erhart[1,*]

[1] *Department of Physics, Chalmers University of Technology, SE-412 96 Gothenburg, Sweden*
[2] *Scientific Computing Department, STFC Rutherford Appleton Laboratory, Didcot OX11 0QX, UK*
[3] *ISIS Neutron and Muon Source, STFC Rutherford Appleton Laboratory, Didcot OX11 0QX, UK*
[*] *erhart@chalmers.se*

# Contents

**S1 NEP model for benzene: Training curves and parity plots** **S2**

**S2 NEP model for hydrogenated Sc-doped $BaTiO_3$: Training curves and parity plots** **S4**

**S3 Path-integral molecular dynamics convergence study for crystalline benzene and hydrogenated Sc-doped $BaTiO_3$** **S5**

**S4 Temperature dependence of Inelastic Neutron Scattering spectrum for crystalline benzene** **S6**

**S5 Red-shift for vibrational spectrum for benzene** **S7**

**References** **S9**

# S1 NEP model for benzene: Training curves and parity plots

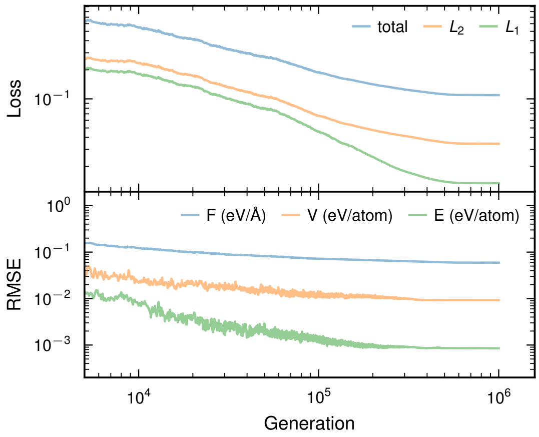


Figure S1: Training curves for the final model for benzene, trained on all available data. This model was used for production runs.

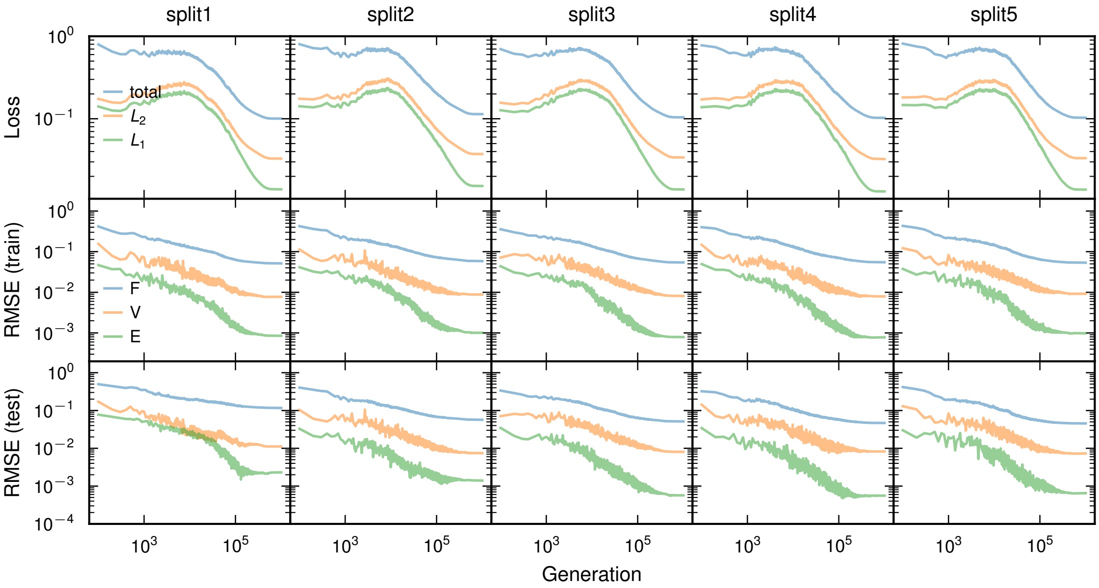


Figure S2: Training curves for the models in the ensemble trained on various K-fold cross validation splits of the training data.

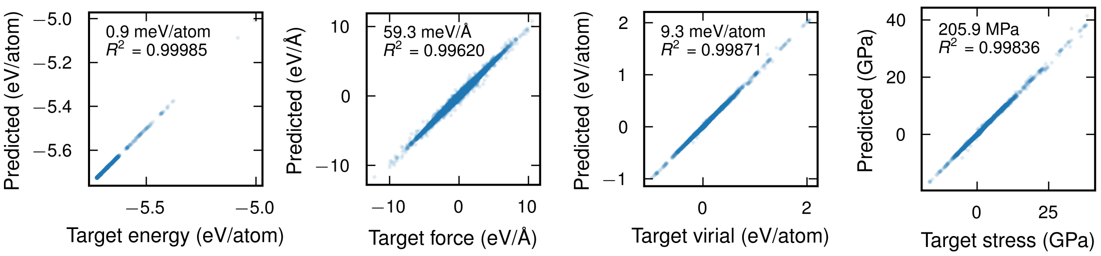


Figure S3: Parity plots for the final benzene model, evaluated on all structures in the data set.

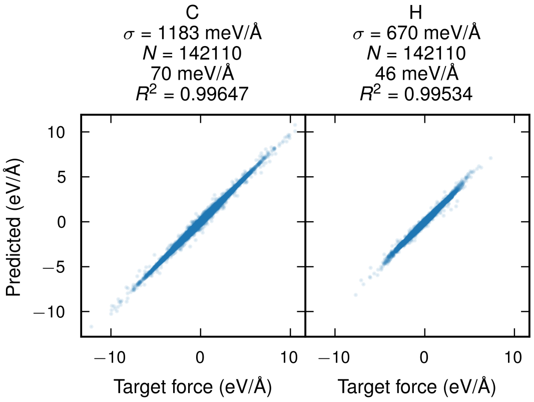


Figure S4: Parity plots for the final benzene model, evaluated on all structures in the data set, split by species. 'C' denotes carbon, and 'H' denotes hydrogen.

## S2 NEP model for hydrogenated Sc-doped $BaTiO_3$: Training curves and parity plots

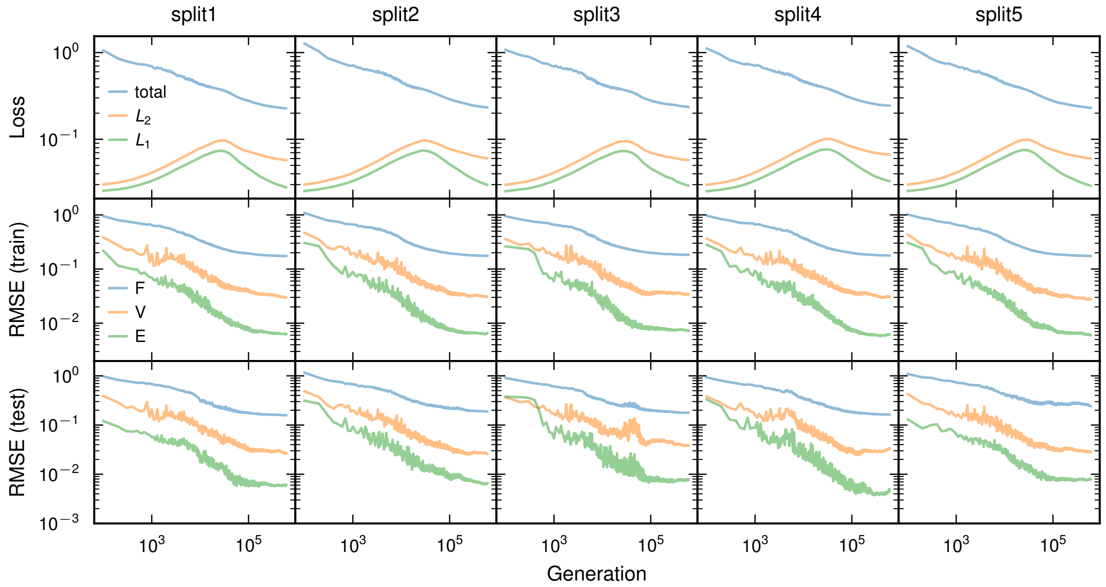


Figure S5: Training curves for the models in the ensemble trained on various K-fold cross validation splits of the training data, for hydrogenated Sc-doped $BaTiO_3$. The 'split1' model was used for production runs.

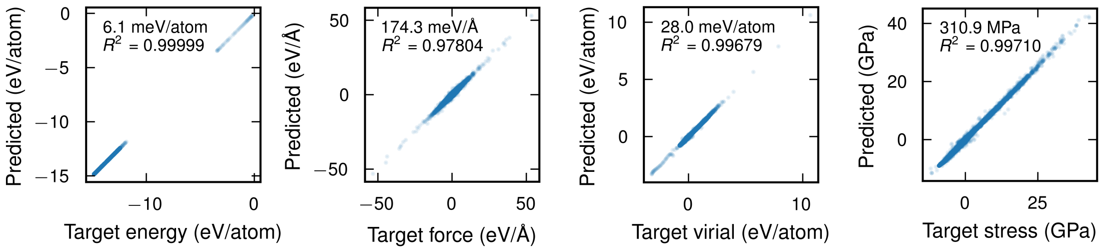


Figure S6: Parity plots for the final hydrogenated Sc-doped $BaTiO_3$ model, referred to as 'split1' in Fig. S5, evaluated on all structures in the data set.

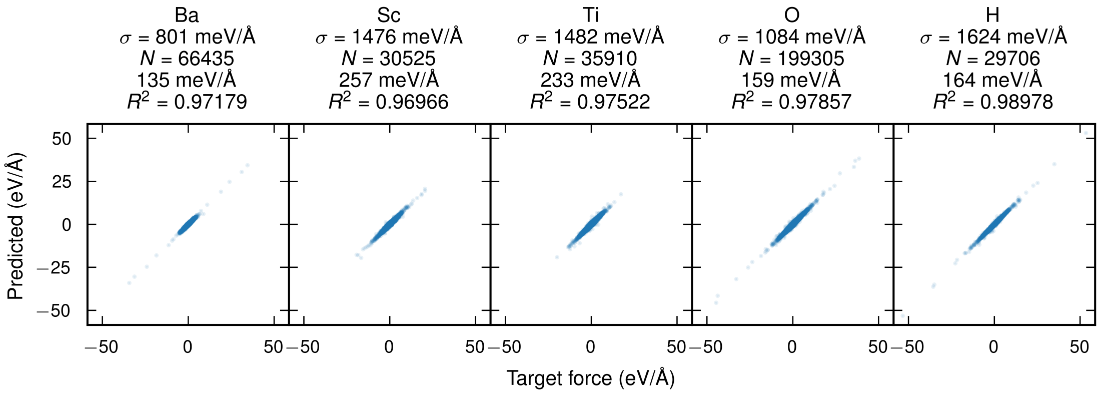


Figure S7: Parity plots for the final hydrogenated Sc-doped $BaTiO_3$ model, referred to as 'split1' in Fig. S5, evaluated on all structures in the data set, split by species.

## S3 Path-integral molecular dynamics convergence study for crystalline benzene and hydrogenated Sc-doped $BaTiO_3$

Here we vary the number of PIMD beads and study the convergence for various properties for crystalline benzene and hydrogenated Sc-doped $BaTiO_3$. For all simulations in this work, we used 32 PIMD beads. The computational cost of a PIMD simulation scales linearly with the number of beams. For benzene, we thus focused our simulations on a temperature of 127 K, since we had available experimental data at that temperature, and the computational cost of performing PIMD with more than 32 beads was deemed too excessive (Fig. S8). For completeness, we include simulations at a range of other temperatures for crystalline benzene compared to experimental data, but note that the number of beads is not necessarily sufficient in all cases (Sect. S4).

For hydrogenated Sc-doped $BaTiO_3$ we performed the convergence study in the hexagonal structure with a Sc doping fraction of 0.16 (Fig. S9). The simulations presented in the main work are performed at 15 K. 32 beads was again used to strike a balance between accuracy and computational cost, but do note that the potential energy and volume of the systems are not fully converged for that number of beads.

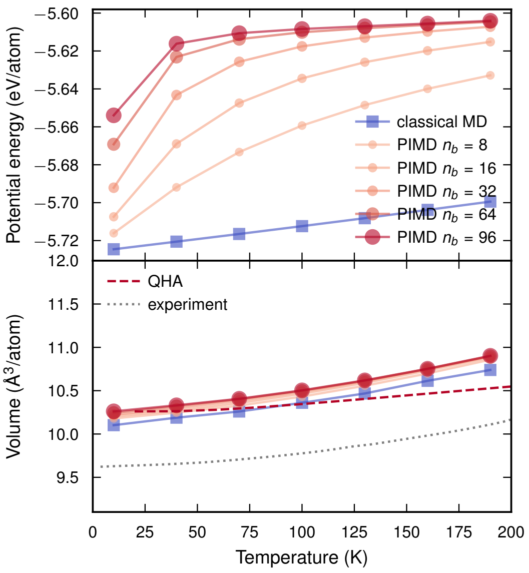


Figure S8: Potential energy and volume from molecular dynamics simulations run in the PIMD ensemble for crystalline benzene.

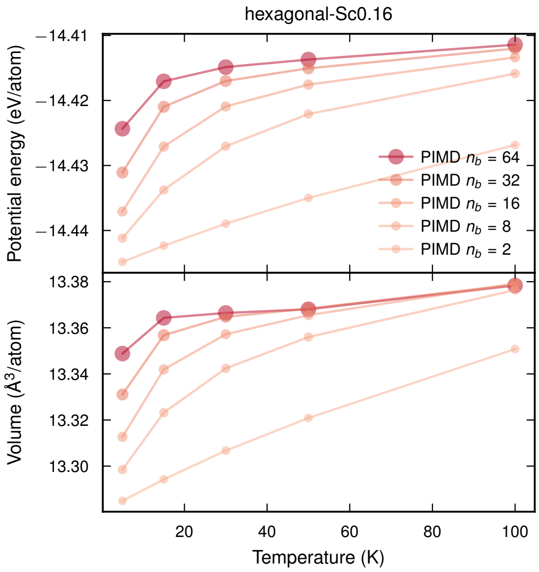


Figure S9: Potential energy and volume from molecular dynamics simulations run in the PIMD ensemble for hydrogenated Sc-doped $BaTiO_3$ in the hexagonal phase with a doping fraction of 0.16.

# S4 Temperature dependence of Inelastic Neutron Scattering spectrum for crystalline benzene

Experimental data compared with simulated spectra at 127 K, 103 K, 75 K, and 24 K. Note that the number of PIMD beads used to perform equilibration is not necessarily enough, see Sect. S3

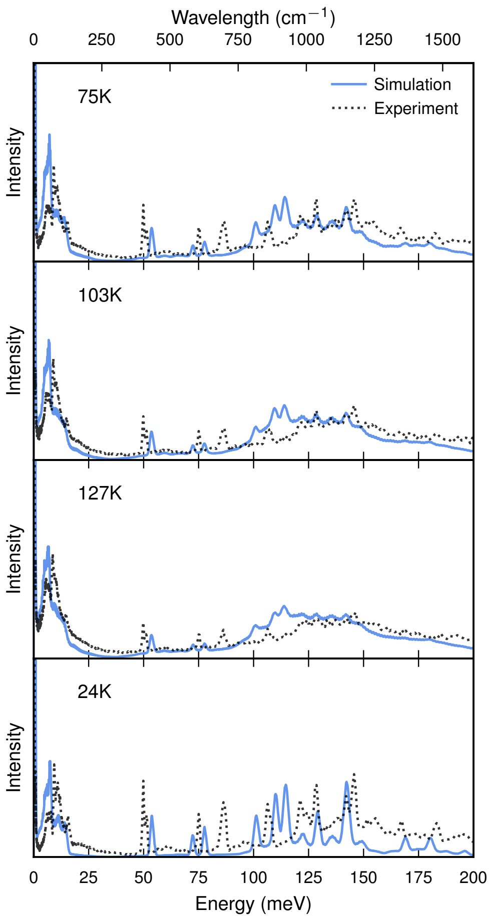


Figure S10: Predicted INS spectrum for crystalline benzene at the TOSCA spectrometer, at 127 K, 103 K, 75 K, and 24 K.

# S5 Red-shift for vibrational spectrum for benzene

The simulated INS spectrum for benzene is red-shifted compared to the experimental spectrum measured at TOSCA. We compare the harmonic density of states (DOS) calculated using our production NEP model for benzene to calculations and experiments performed at low temperature Fig. S11. We focus on the harmonic DOS to decouple the predicted mode energies from the temperature in our MD simulations, as well as the ensemble in which the simulation was conducted in (in this case, NVE). Focusing on the region around 100 meV, we observe that the DOS for our NEP model trained on the vdw-CX functional is red-shifted by approximately 25 meV compared to the collected Raman and IR spectroscopy experiments, as well as the simulated values based on Møller-Plesset perturbation theory (MP2) and DFTMD using a LDA functional. All collected experiments and simulations agree well with the experimental INS spectrum measured at TOSCA. The NEP model used in this work is well-converged with regards to the target energies, forces, and virials calculated using the vdW-CX functional, achieving errors of 8.510 meV atom$^{-1}$ for the energies, 59.29 meV Å$^{-1}$ for the forces, and 9.295 meV atom$^{-1}$ for the virials (Sect. S1). We thus attribute a systematic red-shift of the predicted DOS for our NEP model to be a feature of the vdW-CX functional.

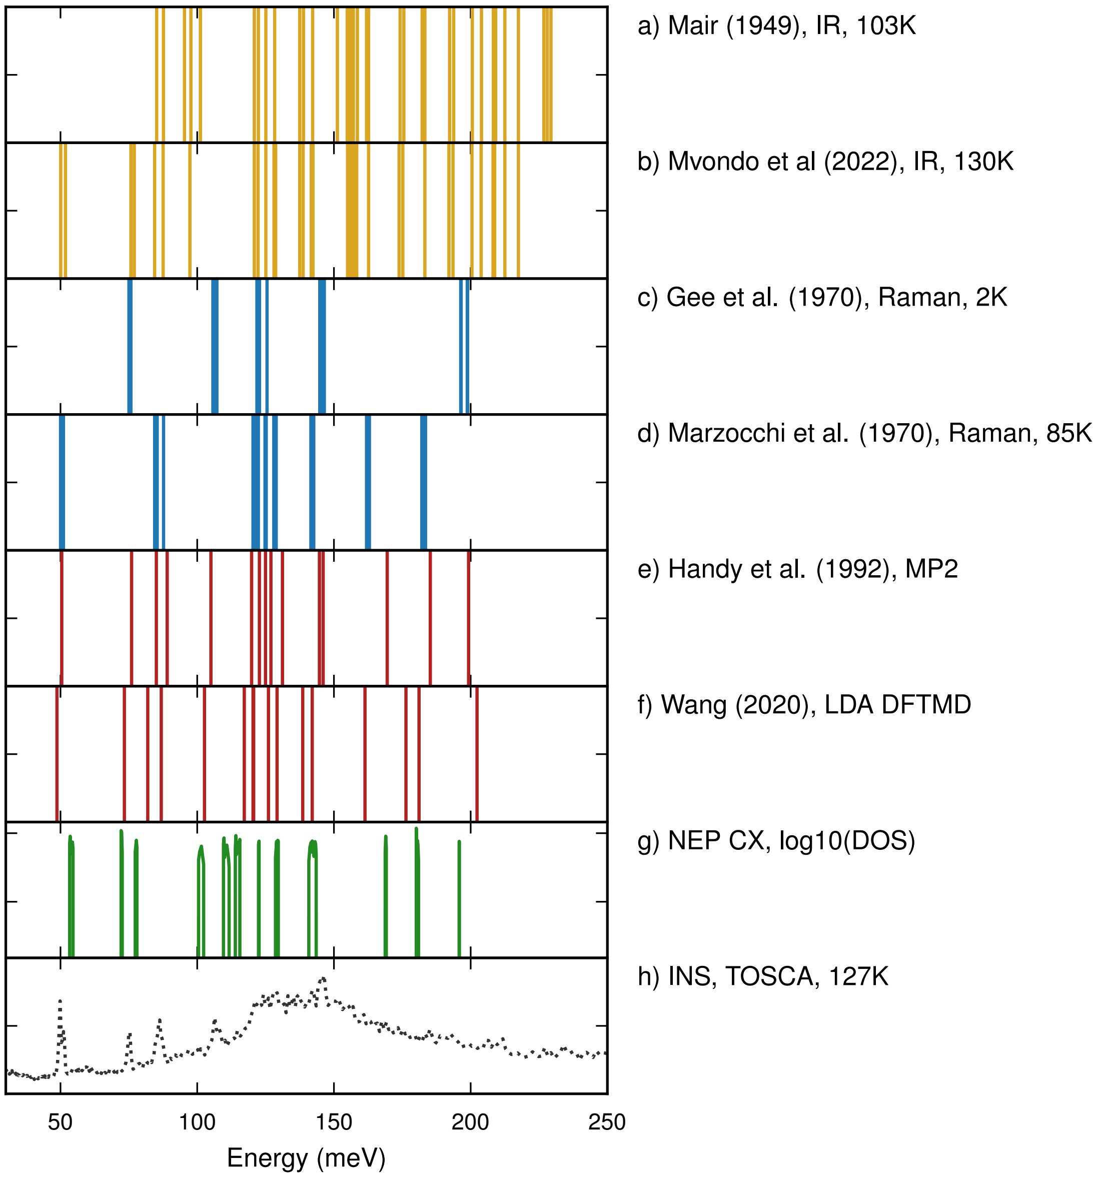


Figure S11: Compilation of density of vibrational frequencies for benzene from the literature. a) IR spectrum measured by Mair et al.[1] b) IR spectrum measured by Mvondo et al.[2] c) Raman spectrum measured by Gee et al.[3] d) Raman spectrum measured by Marzocchi et al.[4] e) Møller-Plesset perturbation theory (MP2) calculations by Handy et al.[5] f) Vibrational modes from DFTMD by Wang et al.[6] g) Harmonic density of states (DOS) computed using the NEP model for benzene developed in the course of the present work. h) Experimental INS spectrum for crystalline benzene measured at TOSCA at 127 K, measured in this work. The experimental results and simulations from the literature generally agree well with our measured INS spectrum in the region around 100 meV, indicating that the red-shift we observe for the our NEP model (g) is related to the DFT-functional used to train the model.

# References

[1] Robert D. Mair and Donald F. Hornig. The Vibrational Spectra of Molecules and Complex Ions in Crystals. II. Benzene. *The Journal of Chemical Physics*, 17(12):1236–1247, December 1949. ISSN 0021-9606. doi: 10.1063/1.1747149. URL https://doi.org/10.1063/1.1747149.

[2] Delphine Nna-Mvondo and Carrie M. Anderson. Infrared Spectra, Optical Constants, and Temperature Dependences of Amorphous and Crystalline Benzene Ices Relevant to Titan. *The Astrophysical Journal*, 925(2):123, February 2022. ISSN 0004-637X. doi: 10.3847/1538-4357/ac350c. URL https://dx.doi.org/10.3847/1538-4357/ac350c.

[3] A. Roger Gee and G. Wilse Robinson. Raman Spectrum of Crystalline Benzene. *The Journal of Chemical Physics*, 46(12):4847–4853, June 1967. ISSN 0021-9606. doi: 10.1063/1.1840646. URL https://doi.org/10.1063/1.1840646.

[4] M. P. Marzocchi, H. Bonadeo, and G. Taddei. Infrared Spectra in Polarized Light of Crystalline Benzene and Benzene-d6. *The Journal of Chemical Physics*, 53(3):867–875, August 1970. ISSN 0021-9606. doi: 10.1063/1.1674151. URL https://doi.org/10.1063/1.1674151.

[5] Nicholas C. Handy, Paul E. Maslen, Roger D. Amos, Jamie S. Andrews, Christopher W. Murray, and Gregory J. Laming. The harmonic frequencies of benzene. *Chemical Physics Letters*, 197 (4):506–515, September 1992. ISSN 0009-2614. doi: 10.1016/0009-2614(92)85808-N. URL https://www.sciencedirect.com/science/article/pii/000926149285808N.

[6] Shaoqing Wang. Intrinsic molecular vibration and rigorous vibrational assignment of benzene by first-principles molecular dynamics. *Scientific Reports*, 10(1):17875, October 2020. ISSN 2045-2322. doi: 10.1038/s41598-020-74872-6. URL https://www.nature.com/articles/s41598-020-74872-6.
